# Supplementary material for: Magnetism and 3D Electron Diffraction Solution of Hydrated Rubidium-Ruthenium Oxide Rb$_2$Ru$_2$O$_7$.H$_2$O
Source: arXiv:2601.13154 source file (2026-01-19)
Supplement: Supplementary file 1 [file diff_SI.tex]

\newenvironment{DIFnomarkup}{}{}
\RequirePackage{shellesc}
\ShellEscape{latexdiff --flatten SI.tex SI_new.tex > SI-d.tex}
\input{SI-d}
\documentclass{dummy} 
